# Supplementary material for: Tensor Random Projection for Low Memory Dimension Reduction
Source: arXiv:2105.00105 source file (2021-04-30)
Supplement: Supplementary file 1 [file appendix_connection2CP.tex]

We can see that $\mathbf{A}$ corresponds to a random low rank tensor of CP rank $k$, $\mathscr{A} = \sum_{j = 1}^k \mathbf{A}_{1,(.,i)} \circ \cdots \circ \mathbf{A}_{N, (.,i)}$, % more notations?? 
where $\circ$ denotes the outer product. The $i^{th}$ row of $\mathbf{A}$ is the vectorization of the $i^{th}$ component of $\mathscr{A}$'s CP decomposition. Therefore, the TRP map is essentially computing the vectorized inner product between $\mathbf{X}$ and each component of a random CP decomposition. In TRP, we find a embedding of $X$ on the space of random low CP rank tensors.
